# Supplementary material for: From Curves to Words and Back Again: Geometric Computation of Minimum-Area Homotopy
Source: arXiv:2309.02383 source file (2023-09-05)
Supplement: Supplementary file 1 [file appendix.tex]

%!TEX TS-program = pdflatex
%!TEX encoding = UTF-8 Unicode
%!TeX spellcheck = en-US
%!TeX root = ..\sosa22.tex

%----------------------- Appendix -------------------------------------
\section{Appendix}
\label{append:appendix}

In this section we provide additional details.
